# Supplementary material for: ReTaSA: A Nonparametric Functional Estimation Approach for Addressing Continuous Target Shift
Source: arXiv:2401.16410 source file (2024-01-29)
Supplement: Supplementary file 1 [file numerical.tex]

% !TEX root = ../nips.tex

\subsection{Datasets and Preprocessing}

Our experiments focus on three datasets: synthetic dataset, UCI 
Communities and Crime Dataset (\citealt{Dua2019}), and Ames Housing Dataset (\citealt{de2011ames}).
\begin{enumerate}
    \item For the synthetic dataset, the data are generated from the model $Y=\X^\top \boldsymbol{\beta}+ \epsilon$, where $\X,\boldsymbol{\beta}\in\mathbb{R}^5$ and $\epsilon \sim \text{Normal}(0,1)$.
    The element values of $X$ are generated from $\text{Normal}(0,1)$. We set up $\boldsymbol{\beta} = [1.132, 2.465, 7.776, 0, 0]^\top$.
    The data with top and bottom $5\%$ response values are filtered.
    \item For UCI communities and crime dataset, the response variable $y$ is the logarithm of the total number of violent crimes per 100K population (\textit{ViolentCrimesPerPop}), and we predict it with the following 7 features.
    \begin{itemize}
        \item the number of vacant households (\textit{HousVacant})
        \item the percent of housing occupied (\textit{PctHousOccup})
        \item the percent of households owner occupied (\textit{PctHousOwnOcc})
        \item the percent of vacant housing that is boarded up (\textit{PctVacantBoarded})
        \item the percent of vacant housing that has been vacant more than 6 months (\textit{PctVacMore6Mos})
        \item the percentage of people 16 and over, in the labor force, and unemployed (\textit{PctUnemployed})
        \item the percentage of people 16 and over who are employed (\textit{PctEmploy})
    \end{itemize}
    \item For the Ames housing dataset, we treat the logarithm of the sale price (\textit{SalePrice}) as the response variable $y$.
    The features are given below.
    \begin{itemize}
        \item linear feet of street connected to property (\textit{Lot Frontage})
        \item Original construction date (\textit{Year Built})
        \item Type 1 finished square feet (\textit{BsmtFin SF 1})
        \item Type 2 finished square feet (\textit{BsmtFin SF 2})
        \item Unfinished square feet of basement area (\textit{Bsmt Unf SF})
        \item Total square feet of basement area (\textit{Total Bsmt SF})
        \item First floor square feet(\textit{1st Flr SF})
        \item Second floor square feet (\textit{2nd Flr SF})
        \item Low quality finished square feet (\textit{Low Qual Fin SF})
    \end{itemize}
\end{enumerate}

We show the marginal distributions of the response variable in each dataset in Figure~\ref{fig.response_distribution}. 

\begin{figure}[ht]
\centering
\includegraphics[width=0.35\linewidth]{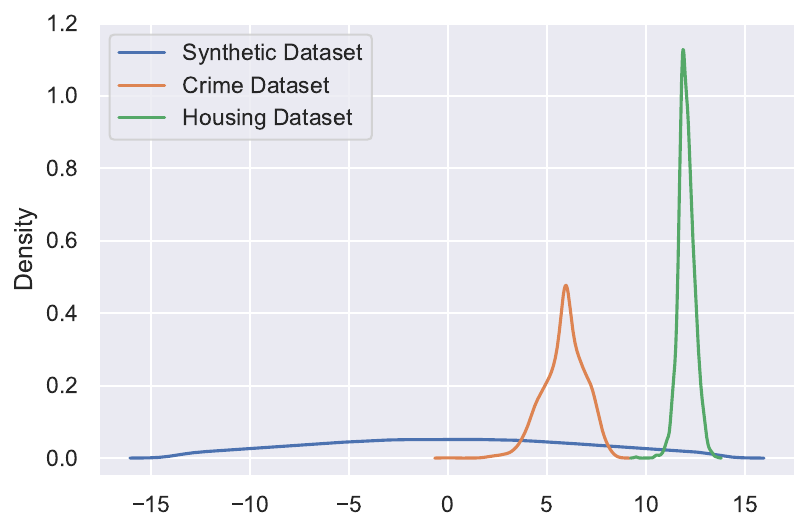}
    \caption{The distributions of response variables in the three experimental datasets}
    \label{fig.response_distribution}.
\end{figure}

\subsection{Target Shift Simulation}

In order to simulate the target shift in our experiments, we adopt a bias sampling scheme to alter the marginal distribution of the response variable, denoted by $Y$. This approach stands in contrast to categorical cases where a Dirichlet distribution suffices for simulating the label shift. Our inverse sampling technique allows us to generate the target shift even when the true underlying distribution of the data is unknown, making it more suitable for real-world datasets.

The response variable $Y_s$ from the source domain is characterized by a cumulative distribution function (cdf) denoted by $F_s(\cdot)$, such that $U_s=F_s(Y_s)\sim\mathrm{Uniform}(0,1)$. If we generate random numbers ${u_{s,1},\dots,u_{s,n}}$ from $\mathrm{Uniform}(0,1)$, we can obtain a sample from the distribution $F_s(\cdot)$ by applying the quantile function $F_s^{-1}(\cdot)$ to ${u_{s,1},\dots,u_{s,n}}$. The strategy for simulating the shift is to generate ${u_{t,1},\dots,u_{t,n}}$ from a distribution that is different from $\mathrm{Uniform}(0,1)$ and recover the shifted sample using inverse sampling: ${F_s^{-1}(u_{t,1}),\dots,F_s^{-1}(u_{t,n})}$. This sampling procedure enables computation of the true importance weight, which is given by $\omega(y)=g_t\left\{F_s(y)\right\}$, where $g_t(u)$ is the probability density function (pdf) of $U_t$ and $f_s(\cdot)$ is the corresponding pdf for $F_s(\cdot)$.

To simulate the target shift, we select $U_t$ to follow a truncated normal distribution between 0 and 1. We replace the unknown function $F_s^{-1}(\cdot)$ with the inverse function of the empirical cdf $\widehat{F}_s(\cdot)$. We present the simulation procedure in Algorithm~\ref{alg:ts}.
The true importance weight is calculated as $\omega(y)=g_t\{\widehat{F}_s(y)\}$, where $g_t(\cdot)$ is the pdf of the selected truncated normal distribution.

\begin{algorithm}
\caption{An Algorithm for Simulating Target Shift}\label{alg:ts}
\KwData{A truncated normal distribution: $\mathrm{TNORM}\langle0,1\rangle(\mu,\sigma)$; a sorted sample $\left\{(\x_i,y_i)\right\}_{i=1}^{N}$ from the source domain so that $y_1\leq\dots\leq y_N$; the sample size of the target sample: $m$.}
\KwResult{A  sample $\{(\x,y)\}$ of size $m$ from the target domain.}
Generate $u_1,\dots,u_m\sim\mathrm{TNORM}\langle0,1\rangle(\mu,\sigma)$\;
\For{$i = 1;\ i \leq m;\ i = i + 1$}{
\For{$j = 1;\ j \leq N;\ j = j + 1$}
{
\If{$j/N\geq u_i$}
{
    Append $(\x_j,y_j)$ to the output\;
    \textbf{break}\;
}
}
}
\end{algorithm}

\subsection{Adaptation Methods Comparison}

In this part, we showcase the effectiveness of our proposed method in mitigating the negative impact of target shift.
In the experiment, we choose the linear regression as both the mapping and prediction models.
We compare our Cores-Adaptation to three existing adaptation strategies: 1) Non-Adaptation, in which the source data trained model is directly applied for the prediction; 2) Oracle-Adaptation, of which the adaptation weight is the ground-truth (i.e., $\omega(y_i) =\omega^*(y_i) =g_t\{\wh F_s(y)\}$); 3) KMM-Adaptation proposed in \cite{zhang2013domain}. Note that, in practice, Oracle-Adaptation is infeasible as the target shift mechanism (i.e., $g_t(\cdot)$) is unknown. In our experiments, we evaluate the adaptation performance with two metrics: 1) Prediction MSE, which the mean square error of the adapted response prediction (i.e. $\sum_{y_i\in \mathcal{D}_t}\|\hat{y}_i - y_i\|^2/|\mathcal{D}_t|$); 2) Weight MSE, which is the mean square error of the estimated adaptation weights v.s. the ground-truth weights (i.e. $\sum_{y_i\in \mathcal{D}_t}\|\hat{\omega}(y_i) - \omega^*(y_i)\|^2/|\mathcal{D}_t|$). Note that, for Non-Adaptation, we calculate the weight MSE by setting $\hat{\omega}(y_i) = 1$ $\forall y_i\in \mathcal{D}_t$.

We start with the setting of $\sigma=0.1$ and study the trade-off between adaptation performance and computation efficiency. 
The experimental results are summarized in Table~\ref{tab.adaptation_comparison}. 
Our results show that Oracle-Adaptation significantly outperforms Non-Adaptation in terms of prediction MSE. Specifically, on the synthetic, crime, and housing datasets, the prediction MSE was reduced by $12.9\%$, $74.6\%$, and $41.9\%$, respectively. These findings strongly suggest that efficient adaptation is crucial for optimal performance.
Both KMM-Adaptation and our Cores-Adaptation can mitigate the negative impact of target shift. 
For example, KMM-Adaptation leads to a $9.6\%$ reduction in prediction MSE on the synthetic dataset, while our Cores-Adaptation achieves an even more significant improvement of $11.0\%$ in prediction MSE.
When considering the weight MSE metric, our Cores-Adaptation consistently outperforms KMM-Adaptation across all three datasets. Specifically, our method achieves a reduction of $59.0\%$, $5.8\%$, and $55.1\%$ on the synthetic, crime, and housing datasets, respectively.
Furthermore, our Cores-Adaptation yields significant improvements in computational efficiency, reducing the per-example computation time from at least $5$ seconds to just $0.2$ seconds when compared to KMM-Adaptation.
\begin{table}[ht]
    \centering
        \caption{The experimental results of adaptation performance and efficiency on the three datasets. The shift parameter $\sigma$ is fixed as 0.1. The numbers reported before and after $\pm$ symbolize the mean and standard deviation, respectively, after trimmed two-side $5\%$ outliers.}
    \label{tab.adaptation_comparison}
    \vspace{.1in}
\begin{tabular}{lc|ccc}
\hline
Dataset & Adaption &  Pred. MSE & Weight MSE &  Time (sec) \\
\hline
 \multirow{4}{*}{Synthetic} 
&Oracle   &  $0.874_{\pm 0.056}$ &  - &  - \\
&None     &  $1.004_{\pm 0.048}$ &  $1.866_{\pm 0.074}$ &  - \\
&KMM      &  $0.907_{\pm 0.065}$ &  $0.593_{\pm 0.441}$ &  $8.984_{\pm 1.928}$ \\
&Cores    &  $0.894_{\pm 0.056}$ &  $0.243_{\pm 0.105}$ &  $0.216_{\pm 0.010}$ \\
\hline
 \multirow{4}{*}{Crime} 
&Oracle   &  $0.116_{\pm 0.007}$ &  - &  - \\
&None     &  $0.457_{\pm 0.043}$ &  $1.803_{\pm 0.086}$ &  - \\
&KMM      &  $0.301_{\pm 0.035}$ &  $1.523_{\pm 0.094}$ &  $6.871_{\pm 1.343}$ \\
&Cores    &  $0.330_{\pm 0.035}$ &  $1.434_{\pm 0.076}$ &  $0.286_{\pm 0.023}$ \\
\hline
 \multirow{4}{*}{Housing} 
&Oracle   &  $0.018_{\pm 0.004}$ &  - &  - \\
&None     &  $0.031_{\pm 0.009}$ &  $1.858_{\pm 0.084}$ &  - \\
&KMM      &  $0.028_{\pm 0.009}$ &  $1.608_{\pm 0.099}$ &  $5.192_{\pm 1.076}$ \\
&Cores    &  $0.026_{\pm 0.009}$ &  $0.722_{\pm 0.196}$ &  $0.209_{\pm 0.044}$ \\
\hline
\end{tabular}

\end{table}

Next, we tune the value of $\sigma$ to investigate the impact of the degree of target shift on the adaptation performance, and the experimental results are shown in Figure~\ref{fig.MSE_over_Sigma}. As the degree of shift increases, the prediction MSEs of the adapted methods are consistently smaller than those from Non-Adaptation. Furthermore, both KMM-Adaptation and our Cores-Adaptation demonstrate similar performance under different degrees of shift. Taking the the computational efficiency into consideration, we can conclude that our Cores-Adaptation provides an effective and efficient approach for mitigating the negative impact of target shift.

\begin{figure}[ht!]
\centering
\begin{tabular}{@{}ccc@{}}
\includegraphics[width=0.32\linewidth]{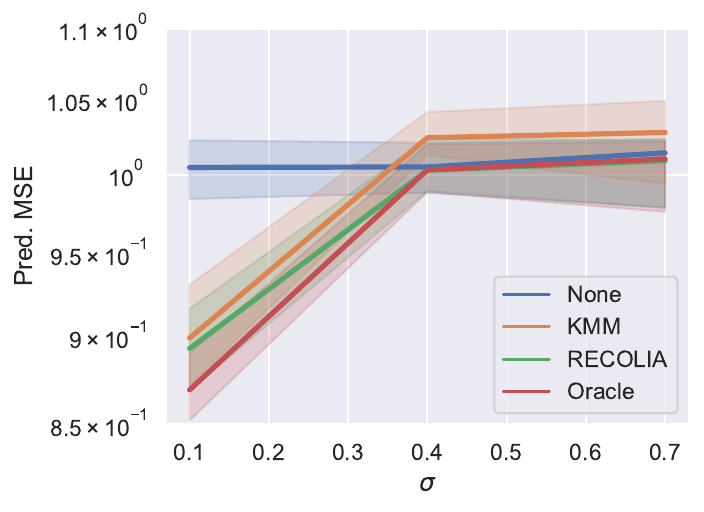} &
\includegraphics[width=0.32\linewidth]{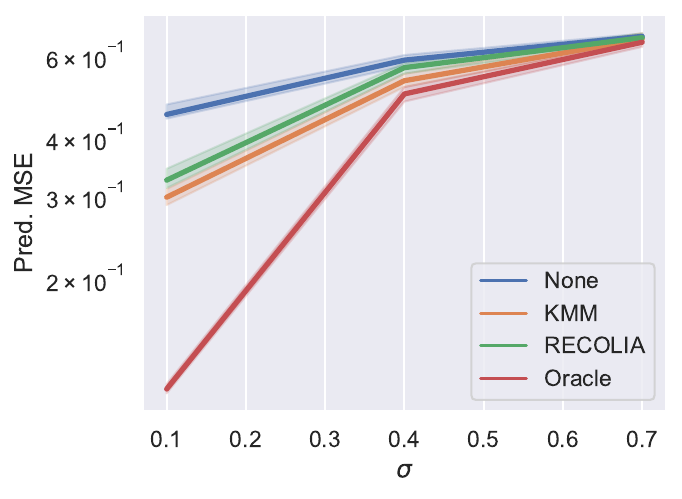} &
\includegraphics[width=0.32\linewidth]{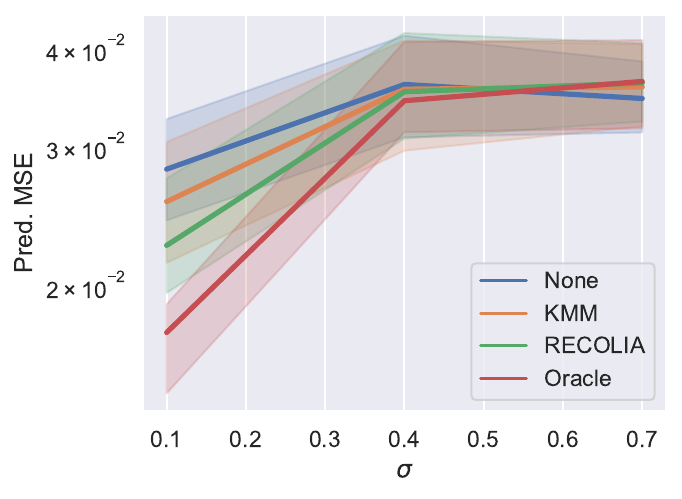}\\
(a) Synthetic Dataset & (b) Crime Dataset & (c) Housing Dataset\\
\end{tabular}
\caption{Prediction v.s. the degree of shift. We control the target shift by adjusting $\sigma$. The solid curves represent the median and the shadow regions are $95\%$ CI error band.}\label{fig.MSE_over_Sigma}
\end{figure}

\subsection{Impact of Mapping Model Choice}

In this experiment, our objective is to assess the impact of mapping model choice on adaptation performance.
We have set the target shift setting to a fixed value of $\sigma = 0.1$, and we will be using the linear regression model for prediction.
To evaluate the impact of mapping model choice, we will compare the performance of different mapping models, including decision tree regression, kernel ridge regression, linear regression, multi-layer perceptron, and random forest regression. 
All these models have been implemented using the "scikit-learn" Python package. 
The multi-layer perceptron model has been set to run with a maximum iteration of 500, while the other mapping models have been left at their default settings.

The experimental results are presented in Table~\ref{tab.model_misspecification}. Our analysis reveals that the random forest model has the lowest weight MSEs across all three datasets, while the overall prediction MSE is roughly similar across different mapping models. Additionally, we observe that smaller weight MSEs generally correspond to smaller prediction MSEs.

\begin{table}[ht!]
    \centering
     \caption{The adaptation performance on the three datasets with different mapping models. The shift parameter $\sigma$ is fixed as 0.1. The numbers reported before and after $\pm$ symbolize the mean and standard deviation, respectively, after trimmed two-side $5\%$ outliers.}
        \label{tab.model_misspecification}
    \vspace{.1in}
\begin{tabular}{lc|cc}
\hline
Dataset & Model &  Pred. MSE & Weight MSE  \\
\hline
 \multirow{5}{*}{Synthetic} 
&Decision Tree           &  $0.914_{\pm 0.053}$ &  $0.127_{\pm 0.047}$ \\
&Kernel Ridge Regression           &  $0.894_{\pm 0.056}$ &  $0.243_{\pm 0.105}$ \\
&Linear Regression                &  $0.894_{\pm 0.056}$ &  $0.243_{\pm 0.105}$ \\
&Multi-layer Perceptron &  $0.890_{\pm 0.057}$ &  $0.189_{\pm 0.080}$ \\
&Random Forest          &  $0.896_{\pm 0.054}$ &  $0.085_{\pm 0.042}$ \\
\hline
 \multirow{5}{*}{Crime} 
&Decision Tree           &  $0.359_{\pm 0.040}$ &  $1.497_{\pm 0.084}$ \\
&Kernel Ridge Regression           &  $0.378_{\pm 0.038}$ &  $1.585_{\pm 0.082}$ \\
&Linear Regression                &  $0.330_{\pm 0.035}$ &  $1.434_{\pm 0.076}$ \\
&Multi-layer Perceptron  &  $0.423_{\pm 0.048}$ &  $1.711_{\pm 0.110}$ \\
&Random Forest           &  $0.297_{\pm 0.036}$ &  $1.311_{\pm 0.095}$ \\
\hline
 \multirow{5}{*}{Housing} 
&Decision Tree           &  $0.027_{\pm 0.009}$ &  $0.946_{\pm 0.163}$ \\
&Kernel Ridge Regression         &  $0.026_{\pm 0.009}$ &  $0.718_{\pm 0.190}$ \\
&Linear Regression                 &  $0.026_{\pm 0.009}$ &  $0.722_{\pm 0.196}$ \\
&Multi-layer Perceptron  &  $0.030_{\pm 0.009}$ &  $1.831_{\pm 0.094}$ \\
&Random Forest           &  $0.025_{\pm 0.009}$ &  $0.612_{\pm 0.174}$ \\
\hline
\end{tabular}
\end{table}

\subsection{Sensitivity Analysis of Regularization}

Our final experiment aims to conduct a sensitivity analysis of the Cores-Adaptation method with respect to the regularization parameter $\alpha$. It is worth noting that a larger value of $\alpha$ will push the estimated adaptation weight towards $1$, while a smaller $\alpha$ will result in larger estimation variation. As in our previous experiments, we fix $\sigma$ to $0.1$ and use linear regression models for both mapping and prediction.

Our experimental results are presented in Figure~\ref{fig.MSE_over_alpha}. The red dashed line in the figure represents the Oracle-Adaptation, which uses the ground-truth weights $\omega^*(y)$ and has zero weight MSEs. The black line denotes the weight MSEs for Non-Adaptation, which is calculated as $\sum_{y_i\in \mathcal{D}_t}|1 - \omega^*(y_i)|^2/|\mathcal{D}_t|$. We range $\alpha$ from 0.01 to 10 for our Cores-Adaptation and show the corresponding weight MSEs using the blue curve. Additionally, we mark the results obtained using the tuned $\alpha$ with a star marker. Our analysis reveals that both very small and very large values of $\alpha$ lead to poor adaptation estimation, as can be observed in Figure~\ref{fig.MSE_over_alpha}(a) and (c). 
While our proposed tuning method can identify a relatively reasonable value for $\alpha$, it is worth noting that the choice of $\alpha$ can be heavily influenced by the properties of the data.
Since finding the best $\alpha$ in all scenarios is a highly non-trivial task, we leave it for future investigation.

\begin{figure}[ht!] 
\centering
\begin{tabular}{@{}ccc@{}}
\includegraphics[width=0.3\linewidth]{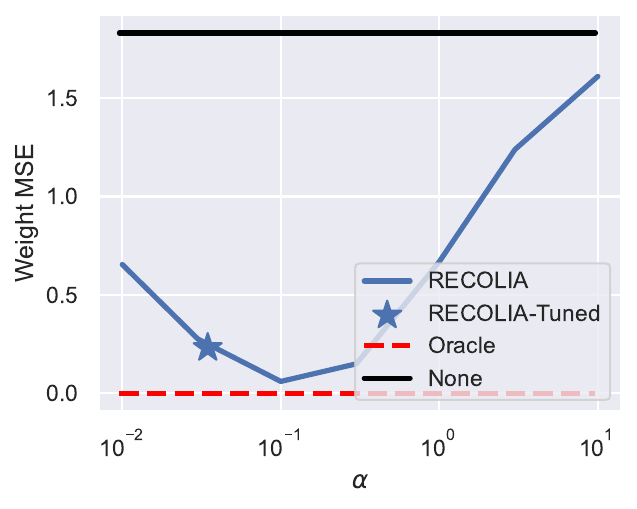} &
\includegraphics[width=0.3\linewidth]{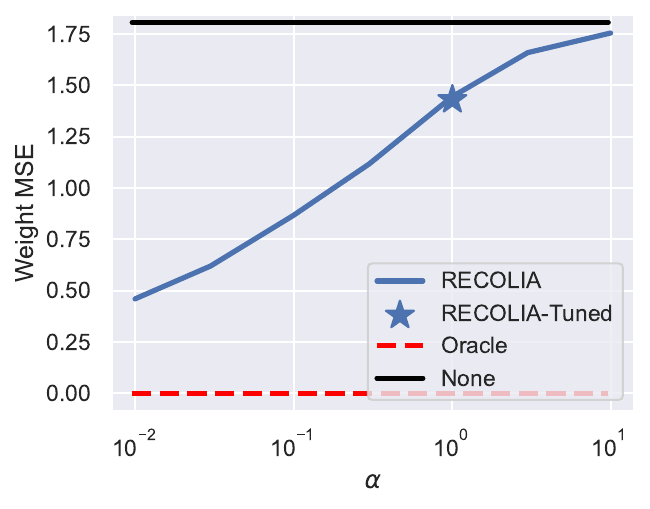} & 
\includegraphics[width=0.3\linewidth]{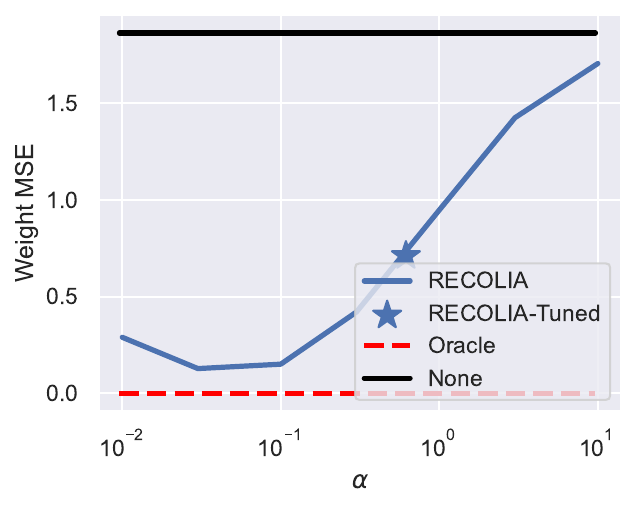}\\
(a) Synthetic Dataset & (b) Crime Dataset & (c) Housing Dataset\\
\end{tabular}
\caption{Weight MSEs v.s. the regularization parameter $\alpha$.}\label{fig.MSE_over_alpha}
\end{figure}
