# Supplementary material for: ReTaSA: A Nonparametric Functional Estimation Approach for Addressing Continuous Target Shift
Source: arXiv:2401.16410 source file (2024-01-29)
Supplement: Supplementary file 3 [file theories_backup.tex]

% !TEX root = ../nips.tex

In this section, we provide a consistency result of our estimator $\hat{\rho}_{\alpha} = \left(\alpha\mathrm{I}+\wh T^\ast\wh T\right)^{-1}\wh T^\ast\wh\eta
$. Namely, we show that $\hat{\rho}_{\alpha}$ converges in probability to $\rho$ under suitable regularization parameter $\alpha$, kernel bandwidth $h$, and function class parameter $\beta$. For the sake of theoretical analysis, in a similar vein as \cite{darolles2011}, we assume $\X \in [0,1]^p$, $y \in [0,1]$, and a joint source density function $p_s(\X, y)$, a source density $p_s(\X)$ and the target density $p_t(\X)$ are all bounded below i.e., $p_s(\X, y), p_s(\X), p_t(\X) \in [\epsilon, \infty), ~\textrm{for some}~\epsilon > 0$, which can be further generalized through some transformations. We also assume that all these densities are $k$-times continuously differentiable, for some $k \in \mathbb{N}$. We list out additional key assumptions we make. 
\begin{assumption}\label{ASSUMP:HS}
The source distribution of $(\X, Y)$ is dominated by the product of its marginal distributions and its density is square integrable with respect to the product of margins. 
\end{assumption}
\begin{remark}
The implication of the assumption \ref{ASSUMP:HS} is that the two operators $T$ and $T^\ast$ defined in \eqref{FORWARD_OPERATOR} and \eqref{ADJOINT_OPERATOR} are Hilbert-Schmidt operators. In particular, the compactness of the operators $T$ and $T^\ast$ directly follows.
\end{remark}

To establish the consistency result, we need to restrict the class of function spaces in which the solution $\rho$ resides in. To this end, we introduce the $\beta$-regularity space of the compact operator $T$ for some $\beta > 0$. 

\begin{definition}\label{beta_regular}
For $\beta > 0$, the $\beta$-regularity space of the compact operator $T$ is defined as 
$$
\Phi_\beta = \left\{\rho \in L^2(Y)~\textrm{such that}~ \sum_{i = 1}^\infty \frac{\langle \rho, \varphi_i \rangle^2}{\lambda_i^{2\beta}} < \infty \right\},
$$
where $(\lambda_i)_{i=1}^\infty$ are the decreasing sequence of nonzero singular values of $T$. Recall that $\{\varphi_i\}_{i = 1}^\infty$  is a set of orthonormal sequences in $L^2(Y)$.
\end{definition}

\begin{remark}
In general, for any $\beta_1 \ge \beta_2$, $\Phi_{\beta_1} \subseteq \Phi_{\beta_2}$. Therefore, the regularity level $\beta$ essentially governs the complexity of the space.
\end{remark}

\begin{assumption}\label{ASSUMP:SOL}
For some $\beta > 0$, we assume that the solution $\rho \in \Phi_\beta$.
\end{assumption}

Finally, we need an assumption on the rate of convergence of kernel-based estimators of $T^\ast$ and $T$. We consider a particular type of kernel constructed as a product of univariate generalized kernel functions, whose definition is given below.

\begin{definition}
    With a bandwidth parameter $h$, a function $K_h: [0,1]^p \times [0,1] \to \mathbb{R}_{\ge 0}$ satisfying 
    \begin{enumerate}
        \item $K_h(x, y) = 0$ if $x \notin [y-1, y] \cap \mathcal{C}$, where $\mathcal{C}$ is a compact interval independent of $y$ and 
        $$
        \sup_{x \in \mathcal{C}, y \in [0,1]} |K_h(x, y)| < \infty
        $$
        \item $h^{-(m+1)} \int_{y-1}^y x^m K_h(x, y)dx = \begin{cases} 
        1 & \textrm{for}~ m = 0, \\
        0 & \textrm{for}~ 1 \le m \le \ell - 1,
        \end{cases}
        $
    \end{enumerate}
    is referred as a univariate generalized kernel function of order $\ell$.
\end{definition}



The assumption on the rate of nonparametric estimators of $T^\ast$ and $T$ based on the generalized kernel functions of order $\ell$ are given below. Its justification can be found in the supplement of \cite{darolles2011}.

\begin{assumption}\label{ASSUMP:kernel}
With a kernel bandwidth parameter $h$ and $\eta = \min\{k, \ell\}$, we assume
\begin{align*}
    ||T^\ast - T||^2 &= O_p\left(\frac{1}{nh^{p+1}} + h^{2\eta}\right), \\
    ||\wh T^\ast - \wh T||^2 &= O_p\left(\frac{1}{nh^{p+1}} + h^{2\eta}\right),
\end{align*}
where $||\cdot||$ is an operator norm.
\end{assumption}

Lastly, we make an assumption on the decaying rate of the bandwidth parameter $h$, given by

\begin{assumption}\label{ASSUMP:bandwidth}
The kernel bandwidth parameter $h$ and satisfies
\begin{equation*}
   \lim_{\substack{h \to 0 \\ n \to \infty}} \frac{\log~n}{n h^{p+1}} = 0
\end{equation*}
\end{assumption}

Before we state the theorem, we first provide preliminary lemmas that we use for the consistency result.

\begin{lemma}\label{LEMMA:kernel_conv}
Under the aforementioned assumptions, our kernel-based approximation of $p_s(\x)$, $p_t(\x)$ denoted by $\wh p_s(\x)$, $\wh p_t(\x)$ satisfies
\begin{itemize}
    \item $\sup_{\x \in [0,1]^p}|\wh p_s(\x)- p_s(\x)| = o_p(1)$
    \item $\sup_{\x \in [0,1]^p}|\wh p_t(\x)- p_t(\x)| = o_p(1)$
\end{itemize}
\end{lemma}
\begin{proof}
    This results follow directly from the Lemma B.1.(i) in the appendix of \cite{darolles2011}.
\end{proof}

\begin{lemma}\label{LEMMA:kernel_denom}
Let $\wh p_s(\x)$ be the kernel-based approximation of the source distribution $p_s(\x)$. Then, 
$$
\frac{1}{\inf_{\x \in [0,1]^p} \wh p_s(\x)} = O_p(1).
$$
\end{lemma}
\begin{proof}
Observe that
$$
|p_s(\x)| \le |p_s(\x) - \wh p_s(\x)| + |\wh p_s(\x)| \Rightarrow |p_s(\x)| - o_p(1) \le |\wh p_s(\x)|,
$$
by Lemma \ref{LEMMA:kernel_conv}. Hence
$$
\inf_{\x \in [0,1]^p}|p_s(\x)| - o_p(1) \le \inf_{\x \in [0,1]^p}|\wh p_s(\x)|.
$$
For a sufficiently large sample size $n$ to construct $\wh p_s(\x)$, we have
$$
\frac{1}{\inf_{\x \in [0,1]^p}|\wh p_s(\x)|} \le \frac{1}{\inf_{\x \in [0,1]^p}|p_s(\x)| - o_p(1)} = \frac{1}{\inf_{\x \in [0,1]^p}|p_s(\x)|} + o_p(1) = O_p(1),
$$
where the first equality holds by the continuous mapping theorem, and the second equality follows from the fact that $p_s$ is bounded away from zero.
\end{proof}

\begin{lemma}\label{LEMMA:SUP_RATE1}
Under the aforementioned assumptions,
$$
\sup_{\x \in [0,1]^p}\left( p_t(\x) - \frac{1}{h^p}\mathbb{E}_s\left(K_{\X, h}(\x-\x_i, \x)\zeta(\x_i) \right) \right)^2 = O(h^{2\eta}),
$$
where $\mathbb{E}_s$ denotes the expectation with respect to the source distribution, $\zeta(\x) = \frac{p_t(\x)}{p_s(\x)}$ and $\eta = \min\{k, \ell\}$.
\end{lemma}
\begin{proof}
Notice
\begin{align*}
\frac{1}{h^p}\mathbb{E}_s\left(K_{\X, h}(\x-\x_i, \x)\zeta(\x_i) \right) &= \frac{1}{h^p}\int_{[0,1]^p} K_{\X, h}(\x-u, \x)p_t(u)du \\ &=\int_{\prod_{i=1}^p[\frac{x_i-1}{h},\frac{x_i}{h}]} K_{\X, h}(hu, \x)p_t(\x-hu)du 
\end{align*}
Using the Taylor expansion of $p_t$ centered at $\x$ , the above is equivalent to 
$$
\int_{\prod_{i=1}^p[\frac{x_i-1}{h},\frac{x_i}{h}]} K_{\X, h}(hu, \x)\left(p_t(\x) + (-h)\sum_{i=1}^p \frac{\partial p_t(\x)}{\partial x_i}u_i + \cdots + \frac{1}{\eta !}\sum_{i_1, \cdots, i_\eta} \frac{\partial^\eta p_t(\x^*)}{\partial x_{i_1}\cdots x_{i_\eta}}(-h)^\eta u_{i_1}\cdots u_{i_\eta}\right)du.
$$
From the definition, boundedness assumption of the generalized kernel function, and continuous differentiability $p_t$, we get
$$
\sup_{\x \in [0,1]^p}\frac{1}{h^p}\mathbb{E}_s\left(K_{\X, h}(\x-\x_i, \x)\zeta(\x_i) \right) = p_t(\x) + O(h^{\eta}),
$$
from which the statement follows.
\end{proof}

\begin{lemma}\label{LEMMA:SUP_RATE2}
Under the aforementioned assumptions,
$$
\left|w(v) - \int_{[\frac{-v}{h}, \frac{1-v}{h}]} K_{Y,h}(hu,v+hu)w(v+hu)du\right|= O(h^\eta),
$$
where $w(y) = \rho(y) + 1 = \frac{p_t(y)}{p_s(y)}$.
\end{lemma}
\begin{proof}
Using the Taylor expansion of $w$ centered at $v$, you have
\begin{align*}
&\int_{[\frac{-v}{h}, \frac{1-v}{h}]} K_{Y,h}(hu,v+hu)w(v+hu)du\\
&= \int_{[\frac{-v}{h}, \frac{1-v}{h}]} K_{Y,h}(hu,v+hu)\left(w(v) + h\frac{\partial w(v)}{\partial v} u + \cdots + \frac{1}{\rho !} \frac{\partial^{\eta}w(v^*)}{\partial v^\eta}h^\eta u^\eta\right)\\
&= w(v) + O(h^\eta),
\end{align*}
where the last equality holds due to the definition, boundedness of the generalized kernel function, and continuous differentiability of $w$.
\end{proof}



\begin{theorem}\label{THM:CONSISTENCY}
Under Assumptions \ref{ASSUMP:HS} - \ref{ASSUMP:bandwidth}, one can show that 
$$
||\hat{\rho}_{\alpha} - \rho ||^2 = O_p\left(\alpha^{\min{(\beta, 2)}} + \left(\frac{1}{nh^{p+1}} + h^{2\eta} \right)\left(1 + \frac{1}{nh^{p+1}} + h^{2\eta} \right)\alpha^{\min{(\beta-2, 0)}} + \frac{1}{\alpha^2}\left(\frac{1}{n} + h^{2\eta}\right)\right).
$$
In particular, under conditions (i) $\alpha \to 0$ with $n \alpha^2 \to \infty$, (ii) $h \to 0$ with $nh^{p+1} \to \infty, nh^{2\eta} \to c < \infty$ and (iii) $\beta \ge 2$ or $nh^{p+1}\alpha^{2-\beta} \to \infty$,
$\hat{\rho}_{\alpha}$ converges in probability to $\rho$.
\end{theorem}

\begin{proof}
Notice $\hat{\rho}_{\alpha} - \rho = R_1 + R_2 + R_3$ where
\begin{align*}
    R_1 &= \left(\alpha\mathrm{I}+\wh T^\ast\wh T\right)^{-1}\wh T^\ast\wh\eta - \left(\alpha\mathrm{I}+\wh T^\ast\wh T\right)^{-1}\wh T^\ast\wh T \rho \\
    R_2 &= \left(\alpha\mathrm{I}+\wh T^\ast\wh T\right)^{-1}\wh T^\ast\wh T \rho - \left(\alpha\mathrm{I}+ T^\ast T\right)^{-1} T^\ast T \rho \\
    R_3 &= \left(\alpha\mathrm{I}+ T^\ast T\right)^{-1} T^\ast T \rho  - \rho.
\end{align*}
We establish upper bounds on the norm of $R_1$, $R_2$, and $R_3$, so as to bound the norm of $\hat{\rho}_{\alpha} - \rho$. First of all, based on proposition 3.2 of the \cite{darolles2011}, we have 
$||R_3||^2 = O(\alpha^{\min(\beta, 2)})$. Secondly, notice that 
\begin{align*}
    R_2 &= \left(\alpha\mathrm{I}+\wh T^\ast\wh T\right)^{-1}\left(\alpha\mathrm{I} + \wh T^\ast\wh T - \alpha\mathrm{I} \right)\rho - \left(\alpha\mathrm{I}+ T^\ast T\right)^{-1} \left(\alpha\mathrm{I} + T^\ast T - \alpha\mathrm{I} \right)\rho \\ 
    &= \left(\mathrm{I} - \alpha\left(\alpha\mathrm{I}+ \wh T^\ast \wh T\right)^{-1}\right)\rho - \left(\mathrm{I} - \alpha\left(\alpha\mathrm{I}+ T^\ast T\right)^{-1}\right)\rho \\
    &= \alpha\left(\alpha\mathrm{I}+ T^\ast T\right)^{-1}\rho - \alpha\left(\alpha\mathrm{I}+ \wh T^\ast \wh T\right)^{-1}\rho.
\end{align*}
We can rewrite 
\begin{align*}
 -R_2 &= \alpha \left(\left(\alpha\mathrm{I}+ \wh T^\ast \wh T\right)^{-1} - \left(\alpha\mathrm{I}+ T^\ast T\right)^{-1}\right)\rho \\    
 &= \alpha\left(\alpha\mathrm{I}+ \wh T^\ast \wh T\right)^{-1} \left(T^\ast T - \wh T^\ast \wh T\right)
    \left(\alpha\mathrm{I}+ T^\ast T\right)^{-1}\rho \\
&= B_1 + B_2,
\end{align*}
where
\begin{align*}
    B_1 &= \alpha\left(\alpha\mathrm{I}+ \wh T^\ast \wh T\right)^{-1} T^\ast \left(T -\wh T\right)
    \left(\alpha\mathrm{I}+ T^\ast T\right)^{-1}\rho, \\
    B_2 &= \alpha\left(\alpha\mathrm{I}+ \wh T^\ast \wh T\right)^{-1} \left(T^\ast - \wh T^\ast \right)\wh T
    \left(\alpha\mathrm{I}+ T^\ast T\right)^{-1}\rho.
\end{align*}
Now we provide a bound on the square of norm of each term in $B_1$ and $B_2$. From \cite{darolles2011, groetsch1984theory}, it is known that
$$
\left|\left|\left(\alpha\mathrm{I}+ \wh T^\ast \wh T\right)^{-1}\right|\right| = O_p\left(\frac{1}{\alpha^2}\right).
$$
From the assumption 1 and 3, we have
\begin{align*}
    ||T^*||^2 &=O(1), \\
    ||\wh T||^2 &\le 2||\wh T - T^*||^2 + 2||T^*||^2 = O_p\left(\frac{1}{nh^{p+1}} + h^{2\eta} + 1\right).
\end{align*}
In addition, note that
\begin{align*}
     \alpha\left(\alpha\mathrm{I}+ T^\ast T\right)^{-1}\rho &= \left(\mathrm{I} - \mathrm{I} + \alpha\left(\alpha \mathrm{I} + T^\ast T\right)^{-1} \right)\rho \\
     &= \left(\mathrm{I}- (\alpha \mathrm{I} + T^\ast T)^{-1}(\alpha \mathrm{I} + T^*T - \alpha \mathrm{I})\right) \rho \\
     &= \left(\mathrm{I} - (\alpha\mathrm{I} + T^\ast T)^{-1}T^\ast T\right)\rho \\
     &= \rho - \left(\alpha\mathrm{I} + T^\ast T\right)^{-1}T^\ast T\rho \\
     &= \rho - \rho_\alpha.
\end{align*}
Again by the assumption 2 and the proposition of 3.11 of the \cite{CARRASCO20075633}, we have
$$
 ||\alpha\left(\alpha\mathrm{I}+ T^\ast T\right)^{-1}\rho|| = O(\alpha^{\min(\beta,2)}).
$$
Therefore, we have
\begin{align*}
    ||B_1||^2 &\le \left|\left|\left(\alpha\mathrm{I}+ \wh T^\ast \wh T\right)^{-1}\right|\right|^2  || T^\ast||^2 ||T-\wh T|| ^2||\alpha\left(\alpha\mathrm{I}+ T^\ast T\right)^{-1}\rho||^2 \\ &= O_p\left(\left(\frac{1}{nh^{p+1}} + h^{2\eta}\right)\alpha^{\min\left(\beta-2, 0\right)} \right), \\
    ||B_2||^2 &\le \left|\left|\left(\alpha\mathrm{I}+ \wh T^\ast \wh T\right)^{-1}\right|\right|^2 ||T^\ast-\wh T^\ast||^2 || \wh T||^2||\alpha\left(\alpha\mathrm{I}+ T^\ast T\right)^{-1}\rho||^2 \\&= O_p\left(\left(\frac{1}{nh^{p+1}} + h^{2\eta}\right)^2\alpha^{\min\left(\beta-2, 0\right)} + \left(\frac{1}{nh^{p+1}} + h^{2\eta}\right)\alpha^{\min\left(\beta-2, 0\right)} \right).
\end{align*}
Combining all together, we get 
\begin{equation*}
    ||R_2||^2 \le 2||B_1||^2 + 2||B_2||^2 = O_p\left(\left(\frac{1}{nh^{p+1}} + h^{2\eta}\right)^2\alpha^{\min\left(\beta-2, 0\right)} + \left(\frac{1}{nh^{p+1}} + h^{2\eta}\right)\alpha^{\min\left(\beta-2, 0\right)} \right).
\end{equation*}
Lastly, we obtain the upper bound on the norm of $R_1$. Note that
$$
||R_1||^2 \le \left|\left|\left(\alpha\mathrm{I}+ \wh T^\ast \wh T\right)^{-1}\right|\right|^2  || T^\ast||^2||\wh\eta - \wh T \rho||^2. 
$$
Recall that $\left|\left|\left(\alpha\mathrm{I}+ \wh T^\ast \wh T\right)^{-1}\right|\right|^2 = O_p\left(\frac{1}{\alpha^2}\right)$ and $||T^*||^2 = O(1)$. To obtain an upper bound on $||\wh\eta - \wh T \rho||^2$, note that
\begin{align*}
    \wh\eta - \wh T \rho &= \wh\eta +1 - (\wh T \rho + 1) \\
    &= \frac{\hat p_t(\x)}{\hat p_s(\x)} - \left(\int_{[0,1]} (\rho(y)+1) \frac{\wh p_s(\x, y)}{\wh p_s(\x)}dy \right) \\
    &= \frac{1}{\wh p_s(\x)}\left(\wh p_t(\x) - \int_{[0,1]}w(y) \wh p_s(\x, y)dy \right),
\end{align*}
where $w(y) = \rho(y) + 1$. Here, $\wh p_t(\x)$ is the KDE estimator for $p_t(\x)$ based on the unlabeled target data, and $\wh p_s(\x)$, $\wh p_s(\x, y)$ are respectively the KDE estimator for $p_s(\x)$, $p_s(\x, y)$ based on the source data. For succinct expressions, we introduce the following notation;
$$
A(\x) = \wh p_t(\x) - \int_{[0,1]}w(y) \wh p_s(\x, y)dy.
$$
One can observe that 
\begin{align*}
    \left |\left| \frac{A(\x)}{\wh p_s(\x)} - \frac{A(\x)}{p_s(\x)}\right|\right| = \left |\left| \frac{A(\x)p_s(\x)-A(\x)\wh p_s(\x)}{\wh p_s(\x) p_s(\x)}\right |\right| \le \frac{\sup_{\x \in [0,1]^p} |p_s(\x) - \wh p_s(\x)|}{\inf_{\x \in [0,1]^p} |\wh p_s(\x)|} \left|\left|\frac{A(\x)}{p_s(\x)}\right|\right|.
\end{align*}
By Lemma \ref{LEMMA:kernel_conv} and \ref{LEMMA:kernel_denom}, we observe that 
\begin{align*}
     \left |\left| \frac{A(\x)}{\wh p_s(\x)} - \frac{A(\x)}{p_s(\x)}\right|\right| = O_p\left(\left | \left |\frac{A(\x)}{ p_s(\x)}\right | \right|\right),
\end{align*}
which gives us 
\begin{align*}
     \left|\left| \frac{A(\x)}{\wh p_s(\x)} \right|\right| = \left|\left| \frac{A(\x)}{p_s(\x)}\right | \right| + O_p\left(\left | \left |\frac{A(\x)}{ p_s(\x)}\right | \right|\right) = O_p\left(\left | \left |\frac{A(\x)}{ p_s(\x)}\right | \right|\right) \Rightarrow ||\wh\eta - \wh T \rho||^2 = O_p\left(\left | \left |\frac{A(\x)}{ p_s(\x)}\right | \right|^2 \right)
\end{align*}
To establish an upperbound of $\left|\left |\frac{A(\x)}{ p_s(\x)}\right | \right|^2$, we decompose $A(\x)$ into
\begin{align*}
    A(\x) = A_1(\x) + A_2(\x) + A_3(\x),
\end{align*}
with
\begin{align*}
    A_1(\x) & = \wh p_t(\x) - \frac{1}{n h^p}\sum_{i=1}^n K_{\X, h}(\x-\x_i, \x) \zeta(\x_i), \\
    A_2(\x) & = \frac{1}{n h^p}\sum_{i=1}^n K_{\X, h}(\x-\x_i, \x) \zeta(\x_i) - \frac{1}{n h^p}\sum_{i=1}^n K_{\X, h}(\x-\x_i, \x) w(y_i), \\
    A_3(\x) & = \frac{1}{n h^p}\sum_{i=1}^n K_{\X, h}(\x-\x_i, \x) w(y_i) - \int_{[0,1]}w(y) \wh p_s(\x, y)dy \\
    &= \frac{1}{n h^p}\sum_{i=1}^n K_{\X, h}(\x-\x_i, \x) w(y_i) - \frac{1}{n h^{p+1}}\sum_{i=1}^n \int_{[0,1]} w(y)K_{Y, h}(y-y_i, y) K_{\X, h}(\x-\x_i, \x)dy\\
    &= \frac{1}{n h^p}\sum_{i=1}^n K_{\X, h}(\x-\x_i, \x) \left(w(y_i) - \frac{1}{ h} \int_{[0,1]} w(y)K_{Y, h}(y-y_i, y)dy\right),
\end{align*}
where $(\x_i, y_i)_{i=1}^n$ are i.i.d. samples of $(\X, Y)\sim p_s$, $\zeta(\x) = \frac{p_t(\x)}{p_s(\x)}$ and $w(y) = \rho(y) + 1 =  \frac{p_t(y)}{p_s(y)}$. Here, $K_{\X, h}$ is the product of $p$ univariate generalized kernel function of of order $\ell$. In a similar fashion, $K_{Y, h}$ is a univariate generalized kernel function of of order $\ell$. . First, we establish the upper bound of $\left|\left|\frac{A_{1}(\x)}{p_s(\x)}\right|\right|^2$. We re-express $A_1(\x)$ into
$$
A_1(\x) = \wh p_t(\x) - p_t(\x) + p_x(\x) - \frac{1}{n h^p}\sum_{i=1}^n K_{\X, h}(\x-\x_i, \x) \zeta(\x_i) = A_{11}(\x) + A_{12}(\x),
$$
where 
\begin{align*}
    A_{11}(\x) &= \wh p_t(\x) - p_t(\x)\\
    A_{12}(\x) &= p_x(\x) - \frac{1}{n h^p}\sum_{i=1}^n K_{\X, h}(\x-\x_i, \x) \zeta(\x_i).
\end{align*}
By the Lemma \ref{LEMMA:kernel_conv} with the continuity and positive lower bound of $p_s(\x)$, we observe that 
$$
\left|\left|\frac{A_{11}(\x)}{p_s(\x)}\right|\right|^2 \le \sup_{\x \in [0,1]^p} |\wh p_t(\x) - p_t(\x)|^2 \left(\int_{[0,1]^p}\frac{1}{p_s(\x)} d\x\right) = o_p(1).
$$
Next, we have
\begin{align*}
    A_{12}(\x)^2 = p_t(\x)^2 - \frac{2 p_t(\x)}{nh^p} \sum_{i=1}^n K_{\X, h}(\x-\x_i, \x)\zeta(\x_i) + \frac{1}{n^2 h^{2p}}\left(\sum_{i,j=1}^n K_{\X,h}(\x-\x_i, \x)K_{\X,h}(\x-\x_j, \x)\zeta(\x_i)\zeta(\x_j) \right),
\end{align*}
which leads to 
\begin{align*}
    \mathbb{E}_s\left(A_{12}(\x)^2\right) &=  p_t(\x)^2 - \frac{2 p_t(\x)}{h^p}\mathbb{E}_s\left( K_{\X, h}(\x-\x_i, \x)\zeta(\x_i)\right) + \frac{n-1}{n h^{2p}}\mathbb{E}_s^2\left(K_{\X,h}(\x-\x_i, \x) \zeta(\x_i)\right) \\ &+  \frac{1}{n h^{2p}}\mathbb{E}_s\left(K_{\X,h}(\x-\x_i, \x)^2 \zeta(\x_i)^2\right) \\
    &\le \left( p_t(\x) - \frac{1}{h^p}\mathbb{E}_s\left( K_{\X, h}(\x-\x_i, \x)\zeta(\x_i)\right)\right)^2 + \frac{1}{n h^{2p}}\mathbb{E}_s\left(K_{\X,h}(\x-\x_i, \x)^2 \zeta(\x_i)^2\right),
\end{align*}
where the expectation is with respect to the source distribution. By the Fubini's theorem, we have
\begin{align*}
\mathbb{E}_s\left(\left|\left|\frac{A_{12}(\x)}{p_s(\x)}\right|\right|^2\right) = \int_{[0,1]^p}\mathbb{E}_s\left(A_{12}(\x)^2\right) \frac{1}{p_s(\x)} d\x.
\end{align*}
Note that, using the change of variables,
\begin{align*}
\frac{1}{nh^{2p}}\mathbb{E}_s\left(K_{\X,h}(\x-\x_i, \x)^2 \zeta(\x_i)^2\right) &= \frac{1}{n} \int_{[0,1]^p} \frac{1}{h^{2p}}K_{\X,h}(\x-u, \x)^2 \frac{p_t(u)^2}{p_s(u)}du\\ &= \frac{1}{n}\int_{\prod_{i=1}^p [\frac{x_i-1}{h^2}, \frac{x_i}{h^2}]} K_{\X,h}(h^2u, \x)^2 \frac{p_t(\x-h^2u)^2}{p_s(\x-h^2u)}du.
\end{align*}
Boundedness of $K_{\x,h}$, continuity and nonzero lower bound of $p_t$ and $p_s$ yields 
$$
\frac{1}{n h^{2p}}\mathbb{E}_s\left(K_{\X,h}(\x-\x_i, \x)^2 \zeta(\x_i)^2\right) = O\left( \frac{1}{n}\right).
$$
Combining with the Lemma \ref{LEMMA:SUP_RATE1}, which states that 
\begin{align*}
    \sup_{\x \in [0,1]^p}\left( p_t(\x) - \frac{1}{h^p}\mathbb{E}_s\left( K_{\X, h}(\x-\x_i, \x)\zeta(\x_i)\right)\right)^2 = O(h^{2\eta}),
\end{align*}
we deduce that 
\begin{align*}
\mathbb{E}_s\left(\left|\left|\frac{A_{12}(\x)}{p_s(\x)}\right|\right|^2\right) = O\left(h^{2\eta} + \frac{1}{n}\right),
\end{align*}
which implies
\begin{align*}
    \left|\left|\frac{A_{12}(\x)}{p_s(\x)}\right|\right|^2 = O_p\left(h^{2\eta} + \frac{1}{n}\right),
\end{align*}
by the Markov inequality. Combining the upperbound of $\left|\left|\frac{A_{11}(\x)}{p_s(\x)}\right|\right|^2$ and $\left|\left|\frac{A_{12}(\x)}{p_s(\x)}\right|\right|^2$, we have 
\begin{equation}\label{UP:A1}
   \left|\left|\frac{A_{1}(\x)}{p_s(\x)}\right|\right|^2 = O_p\left(h^{2\eta} + \frac{1}{n}\right) 
\end{equation}
Next, we establish an upperbound for $\left|\left|\frac{A_{2}(\x)}{p_s(\x)}\right|\right|^2$. Let $\Delta_i = \zeta(\x_i) - w(y_i)$. Then, 
\begin{align*}
\mathbb{E}_s\left(\left|\left|\frac{A_{2}(\x)}{p_s(\x)}\right|\right|^2\right) &= \mathbb{E}_s\left(\left|\left|\frac{1}{nh^p p_s(\x)}\sum_{i=1}^n K_{\X, h}(\x-\x_i, \x)\Delta_i \right|\right|^2 \right) \\
&= \frac{1}{n^2 h^{2p}}\sum_{i\neq j}\int_{[0,1]^p} \mathbb{E}_s(\Delta_i K_{\X, h}(\x-\x_i, \x))\mathbb{E}_s(\Delta_j K_{\X, h}(\x-\x_j, \x))\frac{1}{p_s(\x)}d\x\\
&+ \frac{1}{nh^{2p}}\int_{[0,1]^p} \mathbb{E}_s(\Delta_i^2 K^2_{\X, h}(\x-\x_i, \x))\frac{1}{p_s(\x)}d\x 
%&= \frac{1}{nh^{2p}}\int \mathbb{E}_s(\Delta_i^2 K^2_{\x, h}(\x-\x_i, \x))\frac{1}{p_s(\x)}d\x
\end{align*}
where in the the last equality we used the Fubini's theorem. Now one can show that 
\begin{align*}
\mathbb{E}_s(\Delta_i K_{\X, h}(\x-\x_i, \x)) = \mathbb{E}_{\x_i}\left(\mathbb{E}_{y_i|\x_i}(\Delta_i K_{\X, h}(\x-\x_i, \x))\right) 
= \mathbb{E}_{\x_i}\left(\mathbb{E}_{y_i|\x_i}(\Delta_i) K_{\X, h}(\x-\x_i, \x)\right) = 0
\end{align*}
since 
\begin{align*}
\mathbb{E}_{y_i|\x_i}(\Delta_i) &= \zeta(\x_i) - \int_{[0,1]} \frac{p_t(y)}{p_s(y)}p_s(y|\x_i)dy  = \zeta(\x_i) - \int_{[0,1]} \frac{p_t(\x_i, y)}{p_s(\x_i, y)}p_s(y|\x_i)dy\\ &= \zeta(\x_i) -\frac{p_t(\x_i)}{p_s(\x_i)}\int_{[0,1]} p_t(y|\x_i)dy 
= 0.
\end{align*}
Notice that we used the fact $\frac{p_t(y)}{p_s(y)} = \frac{p_t(\x_i, y)}{p_s(\x_i, y)}$ in the first equality above, which is true by the target shift assumption. Furthermore, 
\begin{align*}
\frac{1}{h^{2p}} \mathbb{E}_s(\Delta_i^2 K^2_{\X, h}(\x-\x_i, \x)) &= \int_{[0,1]}\int_{[0,1]^{p}} \frac{1}{h^{2p}} \left(\zeta(u)-w(y) \right)^2 K^2_{\X, h}(\x-u, \x)p_s(u, y)dudy \\
&= \int_{[0,1]}\int_{\prod_{i=1}^p [\frac{x_i-1}{h^2}, \frac{x_i}{h^2}]} \left(\zeta(\x-h^2u)-w(y) \right)^2 K^2_{\X, h}(h^2u, \x)p_s(\x-h^2u, y)dudy.
\end{align*}
By the boundedness of $K_{\X,h}, p_s, p_t$ and positive lowerbound of $p_s, p_t$, we observe that 
$$
\frac{1}{h^{2p}}\int_{[0,1]^p} \mathbb{E}_s(\Delta_i^2 K^2_{\X, h}(\x-\x_i, \x))\frac{1}{p_s(\x)}d\x = O\left( 1\right).
$$
Combining everything, we get $\mathbb{E}_s\left(\left|\left|\frac{A_{2}(\x)}{p_s(\x)}\right|\right|^2\right) = O\left(\frac{1}{n}\right)$. Again using the Markov's inequality this leads to
$$
\left|\left|\frac{A_{2}(\x)}{p_s(\x)}\right|\right|^2 = O_p\left(\frac{1}{n}\right).
$$
Lastly, to obtain the upperbound of $\left|\left|\frac{A_{3}(\x)}{p_s(\x)}\right|\right|^2$, notice
$$
\mathbb{E}_s\left|\left|\frac{A_{3}(\x)}{p_s(\x)}\right|\right|^2 = \int_{[0,1]^p} \mathbb{E}_s\left(A_3^2(\x) \right)\frac{1}{p_s(\x)}d\x = O\left(\sup_{\x \in [0,1]^p} \mathbb{E}_s \left(A_3^2(\x)\right)\right).
$$ 
Letting 
$$
B(\x_i, y_i) = w(y_i) - \frac{1}{ h} \int_{[0,1]} w(y)K_{Y, h}(y-y_i, y) dy,
$$
we have
$$
A_3(\x) = \frac{1}{n h^p}\sum_{i=1}^n K_{\X, h}(\x-\x_i, \x) B(\x_i, y_i).
$$
Therefore,
\begin{align*}
\mathbb{E}_s\left(A_3^2(\x)\right) &= \mathbb{E}_s\left(\frac{1}{n^2h^{2p}} \left(\sum_{i=1}^n K^2_{\x, h}(\x-\x_i, \x) B^2(\x_i, y_i) + \sum_{i\neq j} K_{\X, h}(\x-\x_i, \x)K_{\X, h}(\x-\x_j, \x) B(\x_i, y_i)B(\x_j, y_j) \right) \right) \\
&= \frac{1}{nh^{2p}}\mathbb{E}(K^2_{\X, h}(\x-\x_i, \x)B^2(\x_i, y_i)) + \frac{n-1}{nh^{2p}}\mathbb{E}^2(K_{\X, h}(\x-\x_i, \x)B(\x_i, y_i)) \\
&\le \frac{1}{nh^{2p}}\mathbb{E}(K^2_{\X, h}(\x-\x_i, \x)B^2(\x_i, y_i)) + \frac{1}{h^{2p}}\mathbb{E}^2(K_{\X, h}(\x-\x_i, \x)B(\x_i, y_i)).
\end{align*}
Using change of variables,
\begin{align*}
&\frac{1}{h^{2p}}\mathbb{E}(K^2_{\X, h}(\x-\x_i, \x)B^2(\X_i, y_i))\\ &= \int_{[0,1]}\int_{[0,1]^p}\frac{1}{h^{2p}}K^2_{\X, h}(\x-u, \x)\left( w(v) - \frac{1}{h}\int_{[0,1]} K_{Y,h}(y-v,y)w(y)dy \right)^2p_s(u,v)dudv \\ 
&=
\int_{[0,1]} \int_{\prod_{i=1}^p [\frac{x_i-1}{h^2}, \frac{x_i}{h^2}]} K^2_{\X, h}(h^2u, \x)\left( w(v) - \frac{1}{h}\int_{[0,1]} K_{Y,h}(y-v,y)w(y)dy \right)^2p_s(\x-h^2u,v)dudv \\
%&= \int_{[0,1]} \int_{\prod_{i=1}^p [\frac{x_i-1}{h^2}, \frac{x_i}{h^2}]} K^2_{\x, h}(h^2u, \x)\left( w(v) - \frac{1}{h}\int_{[0,1]} K_{y,h}(y-v,y)w(y)d y\right)^2p_s(\x-h^2u,v)dudv \\
&= O\left( \int_{[0,1]}\left( w(v) - \frac{1}{h}\int_{[0,1]} K_{Y,h}(y-v,y)w(y)d y\right)^2  dv\right),
\end{align*}
where the last equality holds for any $\x$ due to boundedness of $K_{\x,h}$ and $p_s$ with a positive lower bound of $p_s$. In particular, we have 
$$
\sup_{\x \in [0,1]^p}\frac{1}{h^{2p}}\mathbb{E}(K^2_{\X, h}(\x-\x_i, \x)B^2(\x_i, y_i)) = O\left( \int_{[0,1]}\left( w(v) - \frac{1}{h}\int_{[0,1]} K_{Y,h}(y-v,y)w(y)d y\right)^2  dv\right).
$$
We observe that
\begin{align*}
w(v) - \frac{1}{h}\int_{[0,1]} K_{Y,h}(y-v,y)w(y)d y = 
     w(v) - \int_{[\frac{-v}{h}, \frac{1-v}{h}]} K_{Y,h}(hu,v+hu)w(v+hu)du,
\end{align*}
furthermore, 
\begin{align*}
&\int_{[0,1]}\left( w(v) - \int_{[\frac{-v}{h}, \frac{1-v}{h}]} K_{Y,h}(hu,v+hu)w(v+hu)du\right)^2  dv \\ &\le 2\left(\int_{[0,1]}w^2(v)dv + \int_{[0,1]}\left(\int_{[\frac{-v}{h}, \frac{1-v}{h}]} K_{Y,h}(hu,v+hu)w(v+hu)du\right)^2dv\right) 
\end{align*}

by the boundedness of $K_{Y,h}$, $p_s$, $p_t$ and the positive lower-bounds of $p_s$, $p_t$, we know that the quantity above is bounded and hence,
$$
\sup_{\x \in [0,1]^p}\frac{1}{nh^{2p}}\mathbb{E}_s(K^2_{\x, h}(\x-\x_i, \x)B^2(\x_i, y_i))  = O\left(\frac{1}{n}\right).
$$
To deal with the remaining term, one can observe that
\begin{align*}
&\sup_{\x \in [0,1]^p}\left|\frac{1}{h^{p}}\mathbb{E}_s(K_{\X, h}(\x-\x_i, \x)B(\x_i, y_i))\right| \\&\le \sup_{\x \in [0,1]^p}\int_{[0,1]} \int_{[0,1]^p} \left|\frac{1}{h^{p}}K_{\X,h}(\x-u, \x) \left( w(v) - \frac{1}{h}\int_{[0,1]} K_{Y,h}(y-v,y)w(y)dy \right)p_s(u,v)\right|dudv\\
&= \sup_{\x \in [0,1]^p}\int_{[0,1]} \int_{[0,1]^p} \left|K_{\X,h}(hu, \x) \left( w(v) - \frac{1}{h}\int_{[0,1]} K_{Y,h}(y-v,y)w(y)dy \right)p_s(\x-hu,v)\right|dudv \\
&= O\left(\left| w(v) - \frac{1}{h}\int_{[0,1]} K_{Y,h}(y-v,y)w(y)dy\right|\right) \\
&=  O\left( \left|w(v) - \int_{[\frac{-v}{h}, \frac{1-v}{h}]} K_{Y,h}(hu,v+hu)w(v+hu)du\right|\right)
\end{align*}
where the second to the last equality comes from the boundedness of $K_{\X,h}$, $p_s$ and the positive lower-bounds of $p_s$. From the Lemma \ref{LEMMA:SUP_RATE2}, we know that 
$$
\sup_{\x\in[0,1]^p}\frac{1}{h^{p}}\mathbb{E}_s(\left|K_{\x, h}(\x-\x_i, \x)B(\x_i, y_i))\right| = O(h^\eta).
$$
Therefore, we get
\begin{align*}
  \sup_{\x \in [0,1]^p}\mathbb{E}_s\left(A_3^2(\x)\right) = O\left(\frac{1}{n} + h^{2\eta} \right) &\Rightarrow 
\sup_{\x \in [0,1]^p}
\mathbb{E}_s\left|\left|\frac{A_{3}(\x)}{p_s(\x)}\right|\right|^2 = O\left(\frac{1}{n} + h^{2\eta} \right) \\
&\Rightarrow 
\left|\left|\frac{A_{3}(\x)}{p_s(\x)}\right|\right|^2 = O_p\left(\frac{1}{n} + h^{2\eta} \right)
\end{align*}
Combining altogether, we establish the Theorem 1.
\end{proof}
